# Supplementary material for: Segmentation and Characterization of Macerated Fibers and Vessels Using Deep Learning
Source: arXiv:2401.16937 source file (2024-06-18)
Supplement: Supplementary file 1 [file Supplementary_Material.pdf]

# Deep Learning Approach for Segmentation and Characterization of Fibers and Vessels

Saqib Qamar[a,b], Abu Imran Baba[c], Stéphane Verger[b,c,d], Magnus Andersson[a,b,c]

[a]Department of Physics, Umeå University, Umeå, Sweden
[b]Integrated Science Lab, Department of Physics, Umeå University, Sweden
[c]Umeå Plant Science Centre, Department of Forest Genetics and Plant Physiology, Swedish University of Agricultural Sciences, Umeå, Sweden
[d]Umeå Plant Science Centre (UPSC), Department of Plant Physiology, Umeå University, Umeå, Sweden
[e]Umeå Centre for Microbial Research (UCMR), Umeå, Sweden

## Contents

How to use the model on a Local computer .......... 2
How to use the model on GitHub with Binder .......... 5
Supporting figures .......... 7
How to use the model in a Web application .......... 12

## How to use the model on a Local computer

A step-by-step guide on how to use a trained model to make predictions on a given input image. The source code for the model implementation is available at https://github.com/sqbqamar/fiberseg

### Install Anaconda:

a. Download the Anaconda distribution for operating system from the official website: https://www.anaconda.com/products/distribution
b. Follow the installation instructions for the specific OS (Windows, macOS, or Linux).
c. Make sure you have installed **Python>=3.7** on the system, just select python version during anaconda download.

### Open Spyder IDE:

a. Once Anaconda is installed, you can open the Anaconda Navigator. On Windows, you can find it in the Start menu; on macOS, it's in the Applications folder; and on Linux, you can launch it from the terminal.
b. In Anaconda Navigator, you can click on the **"Launch"** button under the Spyder IDE icon.
c. Alternatively, you can open Spyder directly from the command line (CMD in start menu) by typing **spyder** and pressing Enter.

### Use pip to Install Required Libraries:

**a.** Once you have Spyder open, you can install the necessary libraries by opening a terminal within Spyder. To do this, go to the **"Consoles"** tab in the bottom right panel and click on **"Open an IPython terminal."**
b. In the IPython terminal, you can use the pip command to install the required libraries one by one. pip is a package manager for Python, and it allows you to easily install Python libraries and packages.
c. To install each library, type the following command and press Enter. Replace <library_name> with the name of the library you want to install:

**pip install <library_name>**

Here are the commands for installing the specific libraries which are required:

**For Matplotlib:**
pip install matplotlib>=3.2.2

**For Pillow:**
pip install pillow>=7.1.2

**For Pandas:**
pip install pandas>=1.1.4

**For PyYAML:**
pip install pyyaml>=5.3.1

**For Seaborn:**
pip install seaborn>=0.11.0

**For Requests:**
pip install requests>=2.23.0

**For Scipy:**
pip install scipy>=1.4.1

**For Torch (PyTorch):**
pip install torch>=1.7.0

**For Torchvision:**
pip install torchvision>=0.8.1

**For Tqdm:**
pip install tqdm>=4.64.0

**For Ultralytics:**
pip install ultralytics==8.0.89

Repeat **step c** for each library until you have successfully installed all the required libraries. Once you have completed these steps, we should have Anaconda, Spyder IDE, and all the necessary Python libraries installed on your system. You can now start using these libraries within Python projects.

## Open app.py in Spyder:

Open your **app.py** file in the Spyder IDE from the code directory.

## Import Required Libraries:

Make sure you have the necessary libraries imported at the beginning of your **app.py** file. Add the following import statements to your code:

```
from ultralytics import YOLO
import numpy as np
from PIL import Image
import cv2
import colorsys
import random
import pandas as pd
import os
```

## Navigate to the Directory:

Ensure you are in the correct working directory where your app.py and the trained model file are located. You can navigate to the directory using the **os** module or by setting the working directory in Spyder.

To set the working directory in Spyder:

- Go to the **"File"** menu.
- Select **"Open"** and navigate to your project directory.
- In the **"File Explorer"** tab on the left, right-click on your project directory and choose **"Set console working directory."**

## Load the Trained Model:

Add the following code to load the trained model. Replace **'path/to/your/trained/model'** with the actual path to your trained model file:

**model = YOLO('path/to/your/trained/model')**

## Pass Input to the Model:

To use the model for predictions, you need to pass input data. You can use OpenCV to read an image as input data. Here's an example of how to do this:

**input_data** = cv2.imread('path/to/your/image.jpg') ## **input_data** name is **img** in the code.

**prediction** = model.predict(input_data) ## **prediction** name is **results** in the code.

Make sure to replace **'path/to/your/image.jpg'** with the path to the image you want to process.

## Run the Program:

To run your program, open a command prompt or terminal window and navigate to the directory where your **prediction.py** file is located.

Type the following command to run your program:

**python prediction.py**

### View Results:

After running the program, the segmented results from using the trained model will be displayed.

## How to use the model on GitHub with Binder

To use Jupyter Notebook **(prediction_file.ipynb)** on GitHub with a Binder link, follow these step-by-step instructions:

### Access GitHub Repository:

Start by opening GitHub repository using a github link https://github.com/sqbqamar/fiberseg .

### Click Binder Link:

a. Locate the Binder link which is available in README. It typically appears as a badge.
b. Click on the Binder link. This link will take you to the Binder service.

### Binder Environment Setup:

After clicking the Binder link, Binder will automatically set up a computing environment for Jupyter Notebook. This environment includes the required libraries and packages. This process may take a few moments.

### Launch Jupyter Notebook:

Once the Binder environment is ready, it will open Jupyter Notebook (prediction_file.ipynb) in a web browser.

### Check Model and Image Paths:

In Jupyter Notebook, the first thing you should do is ensure that the paths to trained model file and image are correctly set. You can typically find this information in the first few code cells of the notebook. Verify that the paths are accurate.

### Explore Cell-Wise Code:

You can now explore Jupyter Notebook cell by cell. This is where you will find the code for loading the trained model, passing input data (an image), making predictions, and displaying the results. Examine the code and comments within each cell to understand how the model is used for predictions.

## View the Results:

After you've gone through the cells and made any necessary adjustments to paths or parameters, you can run the cells that perform predictions.

a. Execute the code cells to load the model, pass an input image, and generate predictions.
b. View the results, which visualizes in terms of bounding-box and mask on image.

## Note: It Is Slow Loading

### Environment Creation and Launching Kernel

If the loading time for Jupyter Notebook on Binder is slow, there are a few factors to consider:

- **Binder Server Load:** Binder relies on shared computing resources, and the server load can affect the speed. It is slower during peak times when many users are requesting Binder environments.

- **Internet Connection:** The user's internet connection also impacts loading times.

### Speed Performance:

Unlike GPU, which is designed for parallel processing and is highly efficient for deep learning, CPU is slower in handling computations. So, notebook relies heavily on CPU-based calculations, which can impact processing speed.

# Supporting figures

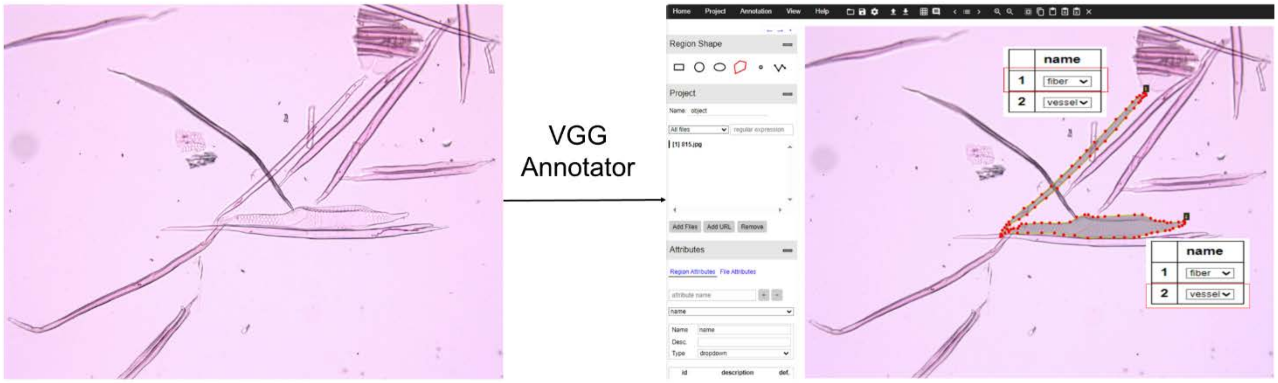


**Figure S1.** The VGG annotator software was utilized for image annotation, where polygon points are drawn over the area of the object to delineate its shape.

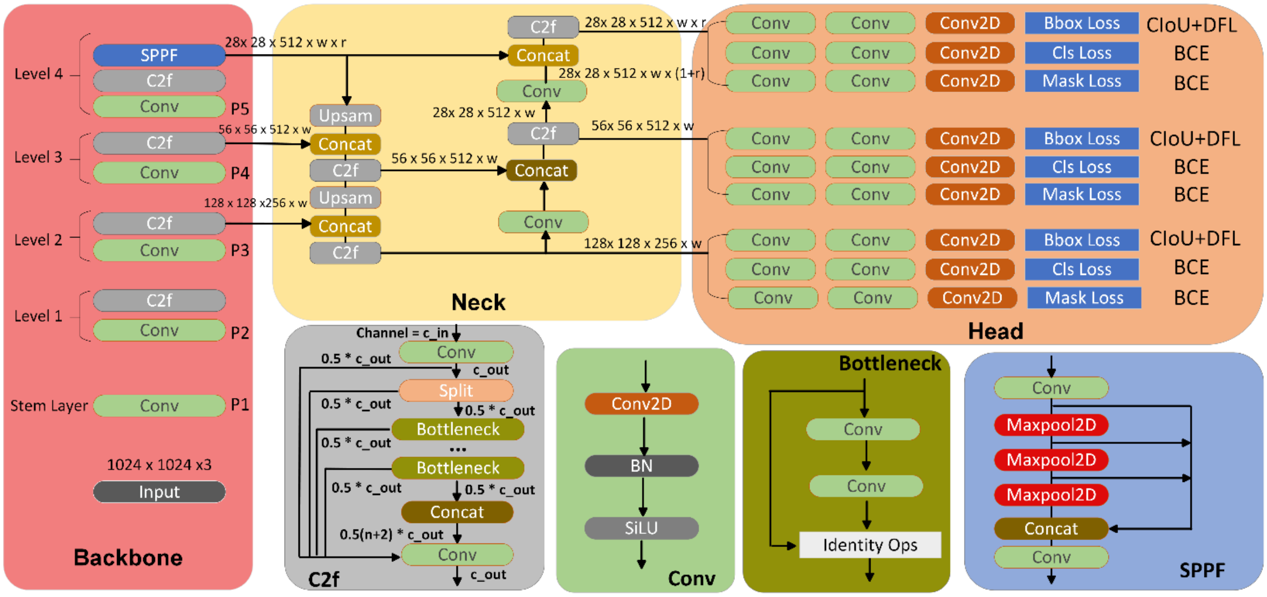


**Figure S2.** YOLOv8 algorithm consists of four main components: Backbone, Neck, Head, and Loss. Backbone incorporates the Cross Stage Partial (CSP) concept that divides the feature map into two parts: one part applies convolutions, while the other part combines its output with the convolutions from the previous part to enhance performance. Unlike YOLOv5, which uses the C3 module, YOLOv8 replaces it with the C2f module. C2f module comprises two Convolutions and multiple BottleNecks connected through Split and Concat operations. Each Convolution in the C2f module consists of Conv-BN-SiLU. This allows YOLOv8 to capture more complete gradient flow information while keeping the model lightweight. Additionally, YOLOv8 reduces computation by decreasing the number of blocks at each stage compared to YOLOv5. In Level 4, YOLOv8 uses the SPPF module as shown in Figure. SPPF is an improved version of Spatial Pyramid Pooling, designed to increase model inference speed.

To address the problem of loss of important information, it is necessary to incorporate a multiscale fusion of features using architectures like FPN (Feature Pyramid Network) and PAN (Path Aggregation Network). The Neck architecture in the Figure fuses features from different scales. Upper features have more details from extra layers. Lower features keep better location details since they have fewer convolutions. YOLOv8 keeps the FPN and PAN structure. But it removes convolutions when upsampling to simplify the model.

YOLOv8 splits classification, detection, and masking into separate branches. YOLOv8 introduces an Anchor-Free approach. This method locates the object based on its center and predicts the distance from the center to the bounding box. The YOLOv8-seg algorithm incorporates classification, regression, and mask branches. To train classification and mask branches, it utilizes the cross-entropy loss to minimize the error and improve its predictions performance in our segmentation tasks. The regression branch incorporates two loss functions, namely Distribute Focal Loss (DFL) and CIoU Loss. The Head architecture encapsulates these approaches in the Figure.

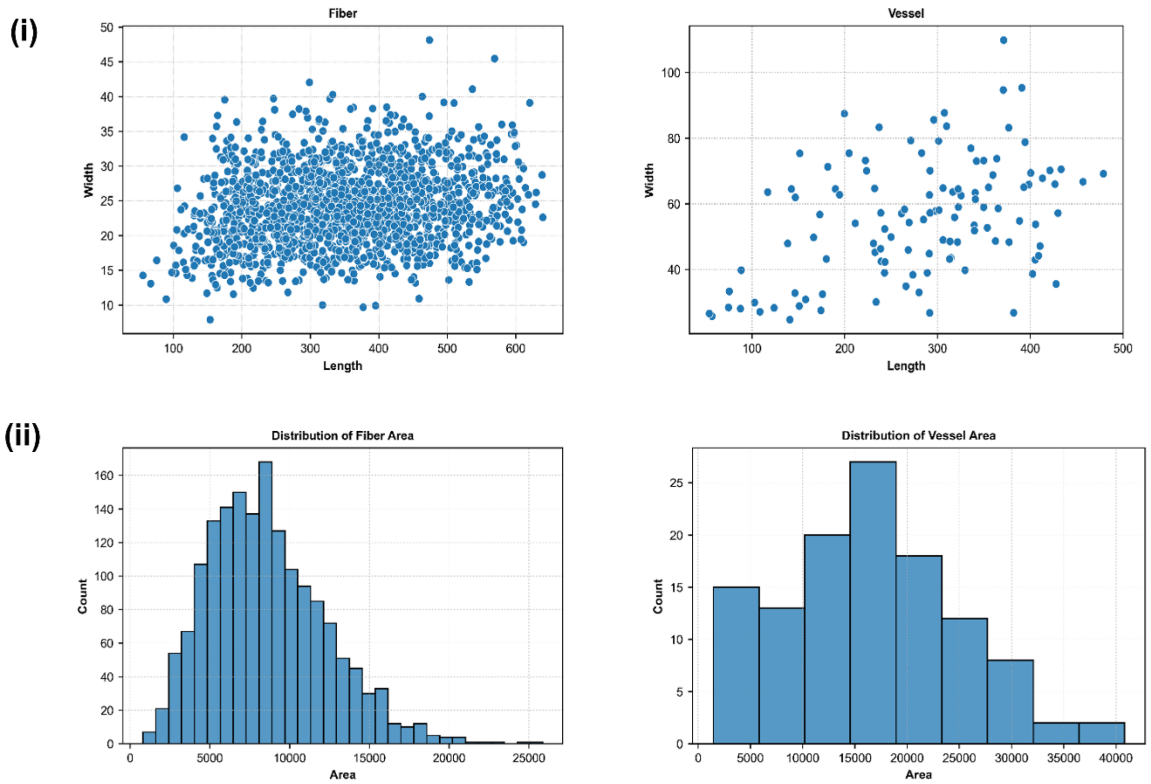


**Figure S3.** Visualizing distributions and relationships of fibers and vessels in 2 large high-resolution (33,384 x 25,1120) images through **(i)** Scatter Plots of length vs width and **(ii)** Histograms of area distributions. In total, 1678 fibers and 117 vessels are detected.

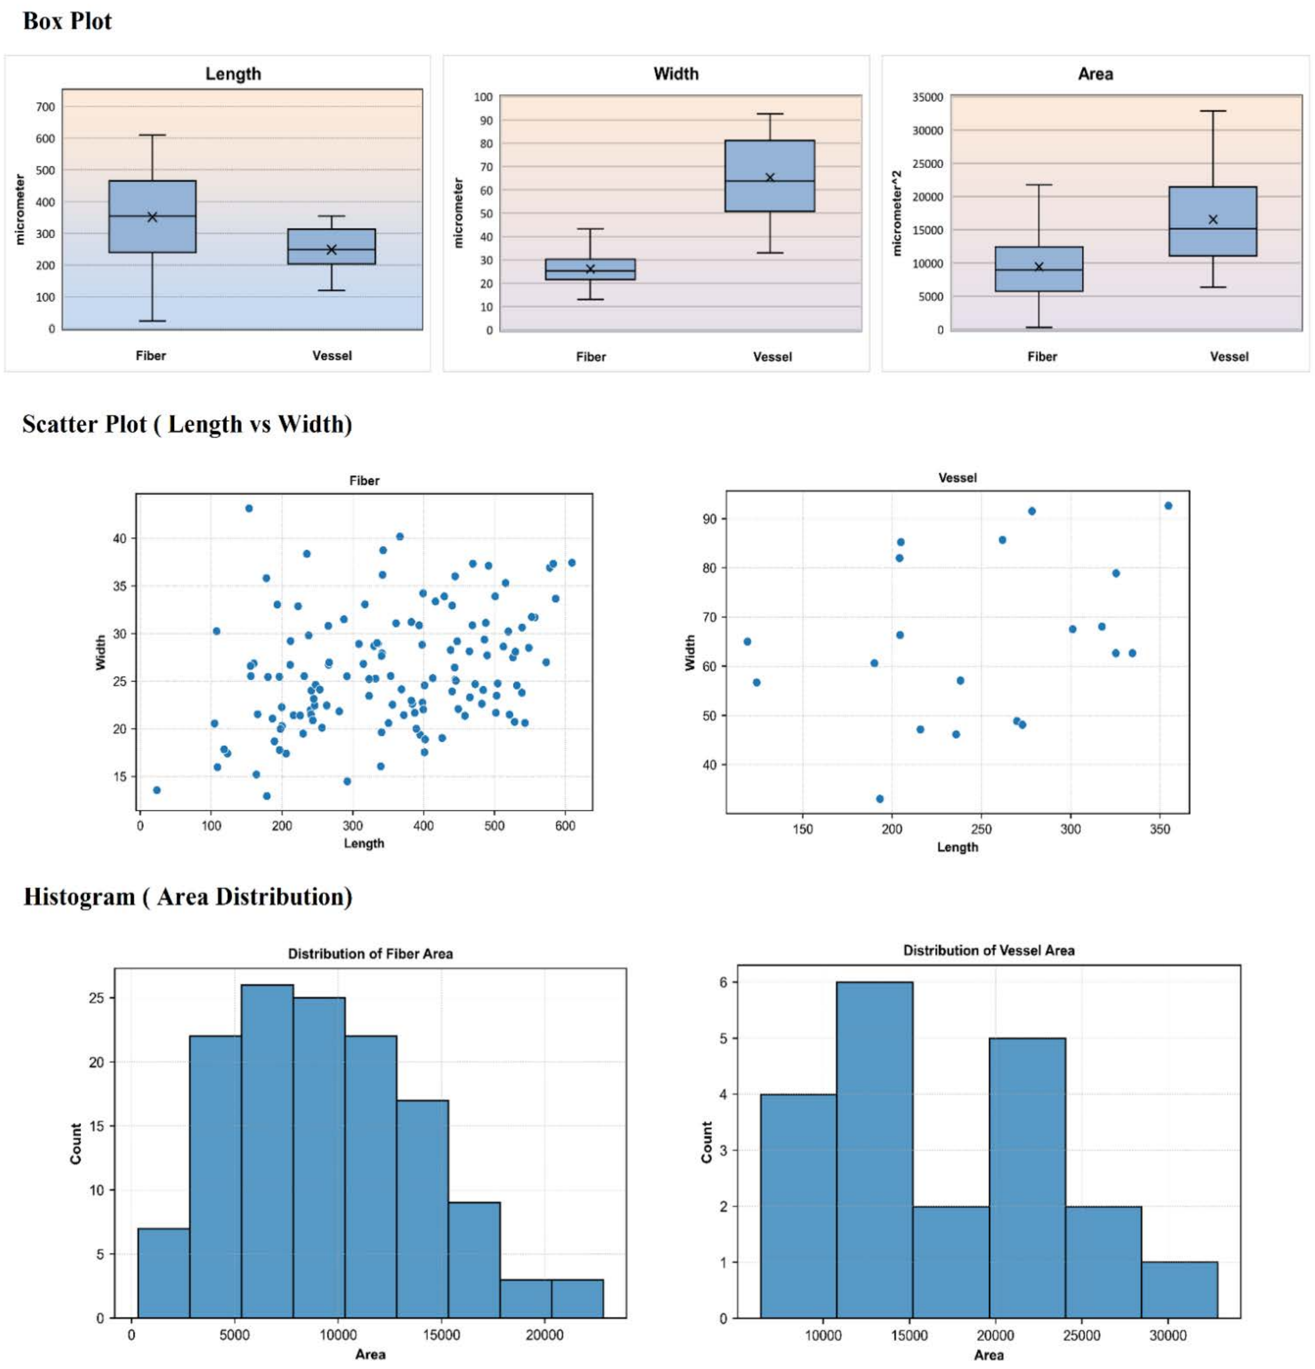


**Figure S4.** Analyzing fiber and vessel distributions in 20 small images (1920 x 1440). The model maintains performance across different image resolutions. This scale invariance is a crucial property for real-world applications, where varying image dimensions will inevitably be encountered. Total detected fibers and vessels are 134 and 20.

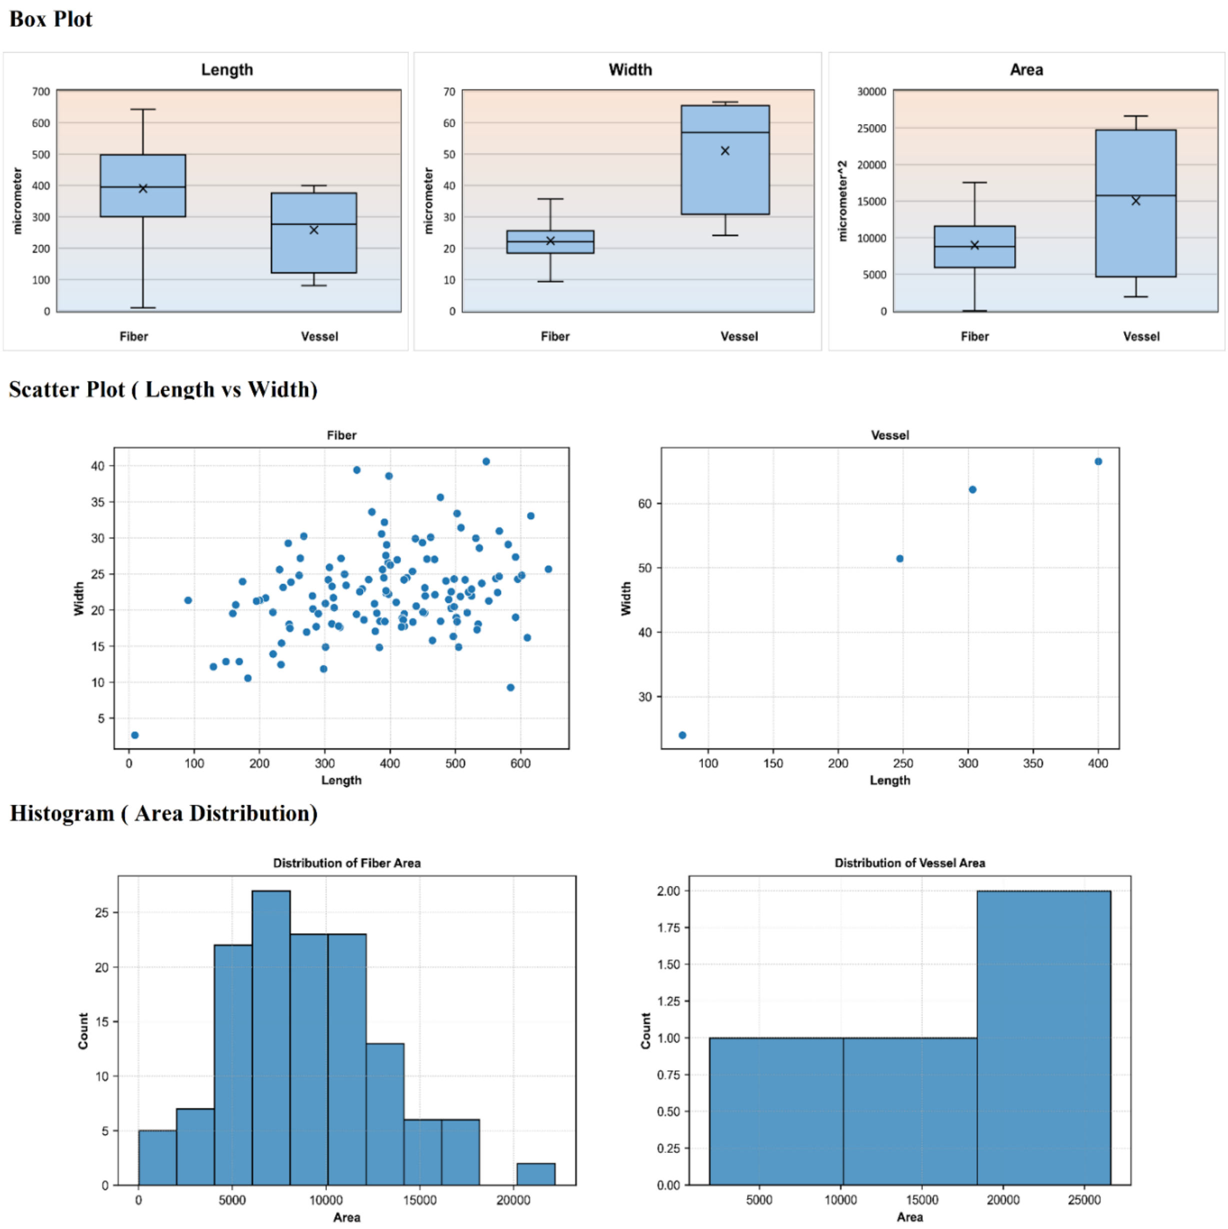


**Figure S5.** Analyzing fiber and vessel distributions in 2 mid-sized images 8275 x 725. The model maintains performance across different image resolutions. This scale invariance is a crucial property for real-world applications, where varying image dimensions will inevitably be encountered. Total detected fibers and vessels are 135 and 4.

# How to use the model in a Web application

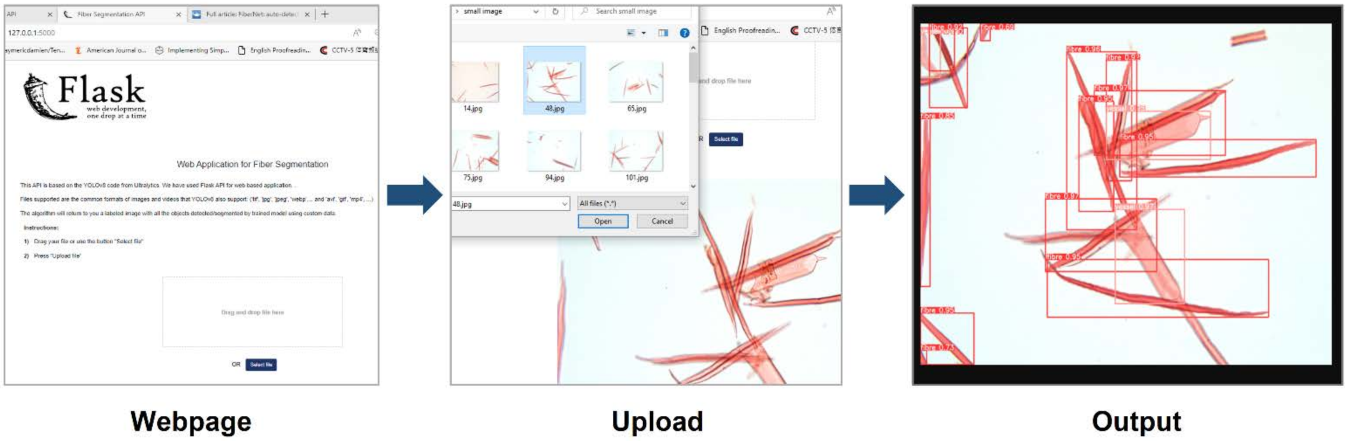


**Figure S6.** Steps in the image show the flow of using application.
